# Supplementary material for: Widescope - A social platform for serious conversations on the Web
Source: arXiv:1111.1958 source file (2011-11-08)
Supplement: Supplementary file 1 [file appendix.tex]

%APPENDICES are optional
%\balancecolumns
\appendix
%Appendix A
\section{Headings in Appendices}
The rules about hierarchical headings discussed above for
the body of the article are different in the appendices.
In the \textbf{appendix} environment, the command
\textbf{section} is used to
indicate the start of each Appendix, with alphabetic order
designation (i.e. the first is A, the second B, etc.) and
a title (if you include one).  So, if you need
hierarchical structure
\textit{within} an Appendix, start with \textbf{subsection} as the
highest level. Here is an outline of the body of this
document in Appendix-appropriate form:
\subsection{Introduction}
\subsection{The Body of the Paper}
\subsubsection{Type Changes and  Special Characters}
\subsubsection{Math Equations}
\paragraph{Inline (In-text) Equations}
\paragraph{Display Equations}
\subsubsection{Citations}
\subsubsection{Tables}
\subsubsection{Figures}
\subsubsection{Theorem-like Constructs}
\subsubsection*{A Caveat for the \TeX\ Expert}
\subsection{Conclusions}
\subsection{Acknowledgments}
\subsection{Additional Authors}
This section is inserted by \LaTeX; you do not insert it.
You just add the names and information in the
\texttt{{\char'134}additionalauthors} command at the start
of the document.
\subsection{References}
Generated by bibtex from your ~.bib file.  Run latex,
then bibtex, then latex twice (to resolve references)
to create the ~.bbl file.  Insert that ~.bbl file into
the .tex source file and comment out
the command \texttt{{\char'134}thebibliography}.
% This next section command marks the start of
% Appendix B, and does not continue the present hierarchy
\section{More Help for the Hardy}
The acm\_proc\_article-sp document class file itself is chock-full of succinct
and helpful comments.  If you consider yourself a moderately
experienced to expert user of \LaTeX, you may find reading
it useful but please remember not to change it.
\balancecolumns
% That's all folks!
